# Supplementary material for: Do LLMs Understand Social Knowledge? Evaluating the Sociability of Large Language Models with SocKET Benchmark
Source: arXiv:2305.14938 source file (2023-12-07)
Supplement: Supplementary file 1 [file 1.appendix.tex]

\section{Experimental setup}

\subsection{Details for training zero-shot models}

% Which models were used?

% What were the resources used?

% What were the training parameters used?

% How were predictions made and evaluated? (e.g., how were span-based and regression tasks evaluates?)
